# Supplementary material for: Quantum Preference Query
Source: arXiv:2405.20429 source file (2024-05-30)
Supplement: Supplementary file 1 [file 8_appendix.tex]

\newpage
